# Supplementary material for: Mediffusion: Joint Diffusion for Self-Explainable Semi-Supervised Classification and Medical Image Generation
Source: arXiv:2411.09434 source file (2024-11-12)
Supplement: Supplementary file 1 [file X_appendix.tex]

% co mozemy dodac
% dataset preparation
% configi dyfuzyjne i enc
% wygrzebac tabelki per klasa? - detailed evaluation with external classifier
% 

% \section{Reproduction details}
% % In this section, we describe details about the reproduction
% \janek{hej Kamil, bo ja to zaczalem juz pisac w Paper for Review.txt, w części appendix i potem wykomentuje po prostu czesc z main submission na czas generacji pdfa}

% \subection{S2MTS2 }
